# Supplementary material for: Geometric friction directs cell migration
Source: arXiv:1310.4129 source file (2013-10-15)
Supplement: Supplementary file 1 [file Leberre-SupMat2.pdf]

**Supplementary Materials to "Geometric friction directs cell migration" by Le Berre et al.**

This section comprises:

I. Supplementary Tables
II. Supplementary movies legends
III. Supplementary Methods Discussion and Model
1. Tilted pillars fabrication
2. Cell culture
3. Migration assay
4. Video-microscopy
5. Movies and Data analysis
6. Statistics
7. Numerical simulation of cell tracks.
8. Discussion on directed cell migration under micro-prisms
9. Discussion on theoretical model
IV. Supplementary References
V. Supplementary Figures and legends
VI. Author contributions

## I. Supplementary Tables

Probability of cells to turn from one direction into another

| After<br>Before | Fwd | Bwd | L | R |
|---|---|---|---|---|
| Fwd | 0 | 63% | 18% | 19% |
| Bwd | 61% | 0 | 21% | 18% |
| L | 39% | 27% | 0 | 34% |
| R | 41% | 24% | 35% | 0 |

**Supplementary Table 1:** Probability of cells to turn from one direction into another. These values correspond to the mean ratios computed over time from distributions shown on Sup. Fig. 4c. The mean is computed for times between 150 min and 400 min.

Simulation parameters

| | |
|---|---|
| Time resolution | 30 s. |
| Total simulation time | 33 h. |

Cell migration parameters

| | Fwd | Bwd | L | R |
|---|---|---|---|---|
| Initial cell direction | 33% | 17% | 15% | 22% |
| Persistence time (min) | 183 | 119 | 118 | 132 |
| Cell mean speed (µm/min) | 0.450 | 0.348 | 0.316 | 0.402 |
| Turning probabilities | See supplementary table 1 | | | |

**Supplementary Table 2:** Parameters used for the numerical simulation of cell migration in a square lattice.

Contribution of each source of bias

| | Mean cell speed (nm/min) | Time spent moving Forward | Time spent moving Backward | Relative Forward increase |
|---|---|---|---|---|
| Control (No bias) | 0.02 | 24.9% | 25.0% | 0.5% |
| All Bias | 104.9 | 41.9% | 24.9% | +68.3% |
| No bias on Persistence time | 54.8 | 33.4% | 29.2% | +14.2% |
| No bias on cell speed | 59.5 | 41.6% | 25.1% | +65.5% |
| No bias on turning probabilities | 78.9 | 33.4% | 21.6% | +54.8% |
| No bias on initial cell direction | 98.4 | 40.8% | 25.2% | +62.6% |
| Experiment | 114.5 | 20.42% | 12.34% | +65.5% |

**Supplementary Table 3:** Contribution of each source of bias in the cell speed and in the time preferentially spent by cells in the Forward direction, deduced from the numerical simulation. In each of the 4 last conditions, one of the 4 biased parameter of the simulation was set to its mean value independently of the direction to test its contribution. It is clear that Persistence time and turning probabilities are the main contributors of the higher time spent in the forward direction; whereas the bias on cell speed impacts only the mean cell speed (highest contributions are in red in the table). Percentages of cells in the Forward and Backward direction are given relatively to the entire population of cells. Each condition of simulation represents a measurement on 10000 virtual cells giving an error margin < 1%.

## II. Supplementary movies legends

**Supplementary Movie 1:** Overlay movie of phase contrast images and HOECHST staining (nucleus, green) of a NHDF cell confined under tilted pillars. Scale bar is 100 µm. Tilt direction is shown with red arrows.

**Supplementary Movie 2:** typical movie showing the body of cells moving under tilted pillars. Original movie was built from phase contrast images where pillars have been removed by substracting to each image a sliding average of 50 frames around the concerned image. Pillars geometry is d = 10 µm; h = 10 µm; alpha = 65 µm, field of view is 0.9x0.67 mm.

## III. Supplementary Methods Discussion and Model

1. Tilted pillars fabrication

The mold used for tilted pillars was done using tilted angle lithography[24]. This method is briefly described below and illustrated in Supplementary Figure 1.

Tilted micropillars were fabricated by casting a pre-polymer solution in a mold also fabricated by casting. First, the designed pattern (micropillars) was produced using a micro-pattern generator (µPG 101, Heidelberg Instruments, Germany) and a Chromium blank mask (Supp. Fig. 1-a). A thin layer of photoresist adhesion promoter (Omicoat, Microchem, Germany) was spin coated on the front side of the Cr mask and baked on a hot plate of 200°C for 1 min. Then, a thin layer of negative photoresist SU-8 (2002, 2005 or 3010) was deposited and soft baked on a hot plate at 65 °C for 1 min then 95 °C for 2 min (Supp. Fig. 1-b). The backside exposure was done with a UV lamp at 365 nm wavelength at incident light angle corresponding to the expected pillars tilt (Supp. Fig. 1-c). The post-exposure bake was done at 65 °C for 1 min then at 95 °C for 2 min. Finally, the resist was developed in SU-8 developer for 1 min with mild agitation, rinsed with isopropyl alcohol and baked at 125 °C for 1 h (Supp. Fig. 1-d).

The master patterns were first replicated by casting a layer of polydimethylsiloxane (PDMS) (Sylgard RTV 184, Dow Corning, USA): trichloromethylsilane (TMCS) was evaporated on the master by chemical vapor deposition. Then, a mixture of PDMS components was poured onto the master, and degassed during 20 min in vacuum (Supp. Fig. 1-e). After curing at 80 °C for 2 hours, the PDMS layer was gently detached, resulting in the first replica of the master. Afterward, the PDMS replica was used as a mold for casting PDMS micropillars in a similar manner (Supp. Fig. 1-f).

2. Cell culture

Primary Normal Human Dermal Fibroblast (NHDF) from the abdominal skin (Biopredic) were cultivated in Dulbecco's Modified Eagle Medium (DMEM/F-12; Gibco) containing 10% Fetal Calf Serum and 1% Penicillin-Streptomycin. Cells were passed every 4 days using Trypsin EDTA (Invitrogen) so that cell confluence remained between 20% and 80%. Cells

were not used above passage 10. For migration experiments, cells were seeded at a concentration of 3000 cells /$cm^2$.

3. Migration assay

3.1. Tilted pillars assay

Cells were cultivated on a 25 mm glass coverslips covered by a thin layer of PDMS. During the fabrication process of these slides, larges pillars (440 µm diameter, 5 µm height, called macro-pillars here to distinguish them from micro-pillars) were molded in the PDMS layer to sustain the PDMS slab containing the tilted micropillars (for fabrication protocol, see [25]). Hence, the cell culture substrate contained large areas 5 µm below the micro-pillars surface, allowing cells to migrate between macro-pillars and the culture substrate (see Supplementary Fig. 3a-b). The coverslips were held in a magnetic observation chamber (Chamlide) retaining culture medium around the sample.
Prior to cell seeding, the PDMS covered surface of the coverslip was incubated for 1 h with a fibronectin solution (50 µg/ml in PBS) and rinsed with PBS. The day after cell seeding, cells were covered by the micro-pillars. For this operation, small PDMS pads (approx. 7 mm x 7 mm x 3 mm) containing tilted micro-pillars on one of their surface were first stuck on a small glass slide (approximately 1 cm x 1 cm) to facilitate handling. Then, the pillars were activated with a plasma cleaner for 30 s at maximum power before being incubated 30 min in a pLL-g-PEG solution (500 µg/mL in 10 mM HEPES, pH 8.6, from SuSoS, Germany) to prevent cell adhesion (NHDFs did not adhere on these surfaces as shown in Supplementary Fig. 2b). Micropillars were incubated in the culture medium for 2h before using them to cover the cells. Cells were incubated for 1h before confinement, with 40 ng/ml HOECHST (Sigma) to stain cell nuclei. The pad containing the pillars was gently deposited in the chamber so that it was floating on the surface of the culture medium. Finally a part of the medium was slowly aspirated with a pipette so that the medium level went below the pad height. At this point, tilted pillars touched cells, and the capillary pressure induced by the medium meniscus pressed slightly the sample on the bottom of the chamber preventing it to move relatively to the culture substrate (Supplementary Fig.3a). Cells were recorded with a video-microscope for 33 hours (see microscopy section).

3.2. Gel Assay

When cell migration was performed between a soft polyacrylamide (PAM) gel and tilted micropillars, the coverslip on which cells were seeded was covered with a flat thin layer of polyacrylamide having a stiffness of 15 kPa and coated with fibronectin. To prepare the gel, the coverslips were first activated with a plasma cleaner for 2 min at maximum power before being incubated in a aminopropyl tri-methoxysilan (APTMS) solution (4% in acetone) for 30 min under sonication. Just before gel deposition, glass slides were further treated with a glutaraldehyde solution (0.5% in PBS) for 30 min for covalent binding of the gel to the glass. To obtain a PAM gel of 15 kPa stiffness, we prepared a gel solution containing 8%vol acrylamide, 0.15 %vol bis-acrylamide, 0.025%wt amonium persulfate solution and 0.05%vol tetramethylethylenediamine (TMED) in an HEPES buffer (10 mM, pH 8.5) according to Boudou *et al.*[26]. A drop of 20 µl of this solution was deposited on a glass slide and covered by the glutaraldehyde treated coverslip. The gel was cross-linked for 45 min before being

removed from the glass slide and rinsed in PBS. The gel was treated to attach fibronectin covalently: 100 µl of Sulfo-SANPAH (1 mM in 10 mM HEPES, pH 8.5) was added to the surface of the gel and activated for 30 s under UV light before being rinsed three times in PBS for 15 min under agitation. Then, the gel surface was covered for 2 hours at 37°C in a fibronectin solution (50 µg/ml in 10 mM HEPES, pH 8.5) before being washed 10 min in PBS. All chemicals were purchased from Sigma Aldrich.

### 3.3. Micro-prism assay

Micro-prisms structures were applied on cells using a cell confiner described in a previous work[25]. Briefly, a 3D mastermold of the structures was done by multi-layer photolithography with SU-8 photoresist (2002 and 2005, Microchem, Germany) using a standard protocol[27]. This master-mold contained, in addition to the micro-prisms shape, the footprint of 440 µm diameter and 3 µm in depth pillars spaced by 1 mm, intended to maintain the space between the textured surface and the culture substrate. A 40 µm thick layer of PDMS maintained on a 10 mm diameter coverslips was molded with these structures. After a 30 s plasma treatment at maximum power, the textured surface was incubated in a pLL-g-PEG solution to prevent cell adhesion. These textured slides were then applied on NHDF cells cultivated in a 35 mm petri dishes by using a custom made device[25] which allowed to gently press the textured slide on the cells with a precision vacuum controller (VG1006, Elveflow, France). Cells were recorded with a video-microscope for 28 hours (see microscopy section).

## 4. Video-microscopy

All time-lapse recordings of cell migration were acquired using a microscope Nikon Eclipse Ti or a ZeissObserver with a temperature control box (adjusted to 37°C), a $CO_2$ stage (adjusted to 5% $CO_2$) and fully equipped by the constructor for live cell fluorescence microscopy. For all experiments intended to be automatically analyzed (see data analysis section), a phase contrast image of the cells and a fluorescence image of the nuclei stained with HOECHST were recorded with a 10x objective every 5 min (Fig1c, supplementary video S1). The DAPI filter set provided by the constructor was used for fluorescence imaging. Image in supplementary figure 3b was acquired with a 60x high NA oil immersion objective on a Nikon confocal spinning disk microscope equipped with a Yokogawa CSU-X1 spinning disk head.

To label pLL-g-PEG, 1 mg of pLL-g-PEG was dissolved into 1 mL 100 mM pH 8.5 NaHCO3 buffer. Then 50 µL 1 mg/mL Alex-594 (Invitrogen) was added and reacted for 2h at room temperature under agitation. Result solutions were then dialyzed for 48 h against 1× PBS to remove unreacted Alex-594 (Slide-A-Lyzer MWCO 3500, Pierce). After that, tilted micro-pillars were treated with plasma and modified with 500 µg/mL pLL-g-PEG-Alexa-594 for 1h, followed by rinsing in PBS. Cell membranes were stained with 40 µg/mL WGA-FITC in cell culture medium for 1h. Afterwards, cell nuclei were stained for 30 min with 5 µM DRAQ5 (Cell signaling Tech.) for confocal imaging.

5. Movies and Data analysis

Timelapse recordings of cells were analyzed using a custom made tracking software written in Matlab. A simplified schematic of the program structure is shown in Supplementary Fig. 6 (letters indicated in the following text refer to this figure).

In a first part, cell paths were automatically tracked from fluorescence images of the Hoechst staining (cell nuclei). Briefly, images were segmented using a watershed method and coordinates of nuclei were defined as the center of mass of the detected nuclei surface (a). Then, cell paths were tracked from one image to another by using an optimization algorithm which selected the best links between images according to a set of parameters like the proximity and the morphological similarity of the detected nuclei (b). Tracks having a duration smaller than 100 data points (which corresponds to 9 h. of migration) where eliminated from the final analyses and tracks having a radius of migration below 20 μm were excluded because they were considered irrelevant to measure the effect of a ratchet having a period of 9 μm (c) (below 60 μm for the micro-prisms experiment). To control the cell behavior, we calculated the mean Mean Square Displacement <MSD> by using the overlapping intervals method[28] (Supplementary Fig. 2d).
Tracks obtained from control cells are very similarly to a Persistent Random Walk (PWR), i.e. persistent at short time ($\langle MSD \rangle \propto t^2$) and random walker at longer time ($\langle MSD \rangle \propto t$). This behavior was expected for fibroblasts, according to the literature[29]. However, at very shot times (i.e. at high frequencies), the moving object did not have a continuous movement (persistent walk) as expected for a normal PWR (blue curve on Supplementary figure 2b). By looking at the power spectral density of the track signal, we observed that nuclei moved following a white noise dominating the signal at frequencies higher than 0.05 $min^{-1}$. This noise, probably due to cytoskeleton contractions might relate to the random component of the force animating the nuclei $\eta(t)$, but did not relate to the persistent motion of the cell at short times. It made the instantaneous speed of migration and instantaneous direction of migration irrelevant regarding to the definition of a PWR (speed and direction were independent of the migration behavior at the time scale of the persistence). To avoid this effect, measured cell tracks were filtered with a lowpass filter having a cutoff frequency of 0.05 $min^{-1}$ (zero shift FIR filter having Gaussian impulse response with a width at mid-height of 15 min) , which removed the high frequency noise, but did not change the path shape at the time scale of the persistence time (d). The filtered tracks were used for analysis (e) shown in Fig 2a-d; 3b-c and Supplementary Fig. 2; 5. Angle histograms were drawn by using a sliding angular window to obtain a smoother representation and identify more precisely the angles of the histogram maxima. For angle histogram representing the direction of migration after a given time, the dataset used to construct histograms was the ensemble of overlapping intervals having a length which corresponds to a given time. Similarly to the angle histogram, graphs representing median speeds depending on the instantaneous speed were drawn by calculating the median of a dataset comprised in a sliding window along the angle parameter. Independently, the position of the pillars was measured from the phase contrast images. First, the angle $\alpha$ and the pitch parameter of the network $L_x$ and $L_y$ were measured by measuring maxima position of the Fourier transform of the image (f). Then, the exact position of the

pattern (the phase parameter $d_x$ and $d_y$) was measured by measuring the position of the maximum of 2D intercorrelation between each image of the video and a reconstructed pattern having the same network parameter $\{L_x, L_y, \alpha\}$ (g). $L_x$, $L_y$, $\alpha$, $d_x$ and $d_y$, were then used to construct a linear transform giving the normalized position in the pattern from the coordinates in the image. This transformation was applied to all points of the cell paths giving the position of the center of mass of the cell nuclei relatively to the structure at any time point (h). The obtained dataset was then sorted to consider only nuclei moving at a speed comprised in a given interval (speed values are given in the graphs) and having a surface comprised between 200 and 266 $\mu m^2$. Nuclear size was filtered for two reasons: i) the model showed that the size of the nucleus was an important parameter governing the bias phenomenon and we expected *a priori* an optimal effect for a restricted range of size. ii) depending on nuclear size, the center of mass is shifted relatively to structures, so that maxima in the distribution of position are scrambled if all sizes are taken into account. Thus, clear maxima in these distribution, appeared only for restricted range of nuclear sizes. The range of size have been chosen to obtain well identified regimes I-III (see theoretical part) and corresponds to nuclei pinched between pillars having a length in the 12-17µm range (slightly longer than the pitch of the pillar network of 10 µm like the one shown in Fig. 1c) (i). Finally, distribution map of the nuclei shown in figures 4b-c were calculated from the sorted data for the different angles of migration. Probabilities of turning from one direction to another shown in supplementary Fig. 4b-c and table 1 were deduced from the angle of migration of the cell relatively to the angle $\alpha$ of tilt direction of the pillar network (j) (Cells were considered to go in one of the 4 direction Fwd, Bwd, L or Right when their direction of migration was in the +/- $\pi/8$ range around these axis). It is to be noted that since the low pass filter applied on the paths altered slightly the real position of the cell, non-filtered data were used to calculate the position distributions. On the contrary, filtered data were used to sort positions according to their angle of migration or speed.

6. Statistics

Proportion of cells going in a specific direction: All data given as a proportion of cell going in in a specific direction are calculated, according to the quadrants shown in supplementary figure 4a, to the ratio between the number of cells fond in quadrant 1 and the number of cells found in quadrant 2 after the given time (The calculus include all intervals of this time found in each paths).

Percentage of decrease of speed: speed bias is given as percentage of decrease of the median speed in slowest direction relatively to the fastest direction. Data points used in this calculus correspond to all data points in all cell paths where the filtered direction of the cell motion was in the +/- $\pi/8$ range around the considered direction.

Percentage of time spent in a specific direction: percentage of time spent in a specific direction corresponds to the percentage of time point in all cell paths where the filtered direction of the cell motion was in the +/- $\pi/8$ range around the considered direction.

Percentage of cells turning in a specific direction: percentage of cells turning in a specific direction given in supplementary Fig 4b correspond to the mean for all incoming direction of

the mean for all times of the proportion of cell which have turned in the given outgoing direction (directly calculated from statistics of turning given in supplementary figure 4c).
Average speed of the population center: the average speed of the population center is calculated as the mean for all time points of instantaneous speed of the mean position of all cells (at the considered time point).

7. Numerical simulation of cell tracks.

To confirm that measurements captured the main aspects of the observed trajectories and are sufficient to explain the direction bias, we numerically simulated cells following a persistent random walk on a square lattice. Numerical simulation of cell migration was performed using a Matlab script (Mathworks) simulating in discrete time the behavior of a group of cells migrating in a square lattice. This simulation hypothesized: i) a constant but direction-dependent cell speed corresponding to the measured median speed (Fig. 2d in the main text); ii) a direction-dependent persistence following a Poisson process and having the measured survival time τ (measured by fitting curves shown in supplementary Fig 4b with exp(-t/ τ)) ; iii) a probability of turning from a specific direction to another one corresponding to the values measured from experimental distributions. (supplementary table 1).

The parameters of the simulation, taken from measurements on experimental data, are given in supplementary table 2. Briefly, for each virtual cell, an initial direction is chosen according to the probability found experimentally after the tilted pillars were put into contact with cells. Then, for each increasing step of time, the coordinates of the cell were updated according to its direction and speed, which changed upon turning. The time between turns is calculated based on a geometric distribution of parameter $p$, where $p = 1 - 2^{-\frac{1}{\tau}}$ corresponded to the probability of turning per unit of time calculated from the experimental persistence time τ (time when half of cells have turned). In case of a turn, the new direction is chosen depending on the current direction according to the measured probability of turning given in the supplementary Table 1. 200 of the obtained tracks are shown in Supplementary Fig. 4d and the mean distribution of the instantaneous direction of migration is given in Fig. 4e for 10000 tracks.

The simulation produced migration paths resembling experimental ones, with a similar bias (Supplementary Fig. 4d and e). Indeed, virtual cells spent 68% more time in the forward direction (65% in experiments) and the average speed of the population center in the direction of the tilt was 105 nm/min (114 nm/min in experiments). To test the role of each source of bias in on parameters of cell tracks, we suppressed independently each source of bias in the simulation and measured its effect on mean cell speed and time spent in each direction (see Supplementary table 3 for the relative contribution of each source of bias). This analysis showed that 3 main phenomena are responsible for most of the direction bias induced by the tilted pillars: i) speed is reduced in the backward direction; ii) cells are more persistent in the forward direction; iii) cells turn more often toward the forward direction.

8. Discussion on directed cell migration under micro-prisms

In this paragraph, we detail the analysis of migration under micro-prisms. To assess that biased migration due to the interaction of the nucleus with the surrounding geometry is not limited to tilted micro-pillars and could apply to any biased geometry, we designed an experiment in which cells are in contact with a surface where series of micro-prisms following each other are engraved (basis, height, depth of prisms were 32 µm, 48 µm and 2 µm respectively). In this experiment, the non-adhesive textured surface is placed 3 µm above the culture substrate, thanks to a recently developed device for cell confinement which allowed to confine cells with a sub-micron precision over large surfaces[25] (see Methods for experimental details). Cells were free to move on the bottom adhesive surface but more confined between the hollow prisms, as illustrated in Supplementary Figure 5a. We recorded cell tracks during 28 h. (Supplementary Fig 5b) and found a significant bias in the migration direction similarly to what was obtained with tilted pillars (see Fig. 3b-c and Supplementary Fig 5c). In this experiment, nuclei concentrated in the hollow prisms where they were less confined (Supplementary Fig 5d). Analysing more precisely the position of nuclei as a function of their direction of migration, we found that nuclei moving toward the basis of the prisms (Bwd direction) concentrated along the basis and glided laterally along this edge (L+R directions). On the contrary, nuclei moving toward the tips (Fwd direction) were distributed more homogeneously along the hollow prism with no apparent accumulation at the tip (Supplementary Fig 5e). To confirm that this absence of accumulation meant that nuclei could pass more easily through the tip tan through the basis of prisms, we measured, for nuclei located close to these barriers, the probability that they keep their initial direction of motion after they moved toward the barrier (Supplementary Fig 5f). As expected, we found that nuclei moving toward the tips were more persistent than nuclei moving toward the basis, indicating that nuclei had more chance to pass the tips than the basis.

9. Discussion on theoretical model

In this paragraph, we present in more details the 1-dimensional model of geometric friction introduced in the main text. We derive explicitly the mean velocity and probability distribution the nucleus of a model cell in an asymmetric landscape, and show that both quantities depend on the direction of motion. These calculations give quantitative support to the observed mechanism of geometric friction.

We consider a cell evolving in a quasi 1–dimensional asymmetric landscape (see Fig. 4a of the main text). The cell motion is assumed to be restricted along the x axis on a flat surface and is confined by a rigid top of periodic asymmetric profile $h(x)$. We consider for modeling purposes a piecewise linear shape of maximum height $h_0$ and minimal height $h_0 - \delta$ where $\delta$ is the maximal indentation such that $\delta \ll h_0$. The period is denoted by $L = a + b$, and the profile $h(x)$ assumed to successively decrease with slope $\delta / a$ over a distance $a$ and then increase with slope $\delta / b$ over a distance $b$. We hypothesize that cell movement is mainly impaired by the nucleus, which has to deform to pass through the successive bottlenecks. The nucleus is assumed to be a spherical linear elastomer of equilibrium radius $R$ and Young modulus $E$. The

profile $h(x)$ is chosen here for the sake of simplicity so that $h_0 - \delta < 2R = h_0$. Using classical results of Hertz[19,20], one finds that the elastic deformation imposed by the geometry leads to an elastic energy stored in the nucleus that writes $U_E = CE\sqrt{R}(2R - h(x))^{5/2}$, where $C$ is an unimportant numerical constant.

An important quantity is the maximal variation $\Delta U_E = CE\sqrt{R}\delta^{5/2}$. We next assume that the cell is polarized and exerts an active force $F_a$ on the nucleus that writes $F_a = \pm F + \eta(t)$ where $F$ is a positive constant, ± denotes the direction of motion (+ and – corresponding here to the Fwd and Bwd directions defined in the main text) and $\eta(t)$ is a random force characterized by $\langle \eta(t)\eta(t')\rangle = 2\Gamma\delta(t - t')$, where $\Gamma$ is the noise amplitude (correlations are here implicitly neglected) . The dynamics of the position $x(t)$ of the nucleus then reads in the over damped regime:

$$\lambda d_t x = \pm F - \partial_x U_E + \eta = -\partial_x U_T^{\pm} + \eta \qquad (1)$$

where $U_T^{\pm} \equiv U_E \pm Fx$ and $\lambda$ has dimension of a friction and is assumed independent of $x$. The dynamics of the nucleus is therefore equivalent to the one of a Brownian particle in a tilted periodic potential. The corresponding Fokker-Planck equation satisfied by the probability density $P(x,t)$ of finding the nucleus at position $x$ at time $t$ reads[21]):

$$\frac{\partial P_{\pm}}{\partial t} = \frac{1}{\lambda}\frac{\partial}{\partial x}\left(\partial_x U_T^{\pm} + \frac{\Gamma}{\lambda}\frac{\partial}{\partial x}\right)P_{\pm} \equiv -\frac{\partial J_{\pm}}{\partial x} \qquad (2)$$

We now look for stationary solutions $P_{\pm}(x)$, which are obtained readily by noticing that $J_{\pm}$ is constant. We introduce $I_p^{\pm}(x) = \int_0^x \exp\left(\lambda U_T^{\pm}(x)/\Gamma\right)$ and $I_m^{\pm}(x) = \int_0^x \exp\left(-\lambda U_T^{\pm}(x)/\Gamma\right)$. It is then found that

$$P_{\pm}(x) = e^{-\lambda U_T^{\pm}(x)/\Gamma}\left[N_{\pm} - \frac{\lambda^2 J_{\pm}}{\Gamma} I_p^{\pm}(x)\right] \qquad (3)$$

where

$$\lambda J_{\pm} = \frac{\Gamma\left(1 - e^{\mp\lambda LF/\Gamma}\right)}{I_p^{\pm}(L) I_m^{\pm}(L) - \left(1 - e^{\mp\lambda LF/\Gamma}\right)\int_0^L e^{-\lambda U_T^{\pm}(x)/\Gamma} I_p^{\pm}(x)dx} \qquad (4)$$

and

$$N_{\pm} = \frac{\lambda^2 J_{\pm} I_p^{\pm}(L)}{\Gamma\left(1 - e^{\mp\lambda LF/\Gamma}\right)} \qquad (5)$$

The mean velocity is then given by

$$v^{\pm} = LJ_{\pm} \qquad (6)$$

These explicit expressions of $v^{\pm}$ and $P_{\pm}(x)$ make possible the identification of the 3 regimes (I-III) introduced in the main text, and have been used to produce the theoretical curves of Fig. 4. In particular the ratio $v^{+}/v^{-}$ (see Fig. 4e) is found to be much larger than 1 in the regime $\Delta U_E \sim FL$ (regime II), resulting in an effective geometric friction as we state in the main text.

## IV. Supplementary References


24. Han M, Lee W, Lee S-K, Lee SS. 2004. 3D microfabrication with inclined/rotated UV lithography. *Sensor Actuat. A-Phys* 111(1):14-20. doi:10.1016/j.sna.2003.10.006.
25. Le Berre M, Aubertin J, Piel M. 2012. Fine control of nuclear confinement identifies a threshold deformation leading to lamina rupture and induction of specific genes. *Integr Biol* 4(11):1406-1414. doi:10.1039/c2ib20056b.
26. Boudou T, Ohayon J, Picart C, Tracqui P. 2006. An extended relationship for the characterization of Young's modulus and Poisson's ratio of tunable polyacrylamide gels. *Biorheology* 43:721-728.
27. del Campo A, Greiner C. 2007. SU-8: a photoresist for high-aspect-ratio and 3D submicron lithography. *J Micromech Microeng* 17:R81- R95. doi:10.1088/0960-1317/17/6/R0
28. Dickinson RB, Tranquillo RT (1993) Optimal Estimation of Cell Movement Indices from the Statistical Analysis of Cell Tracking Data. *AIChE Journal* 39(12):1995-2010.
29. Gail MH, Boone CW (1970) The locomotion of mouse fibroblasts in tissue culture. *Biophys J* 10(10):980-993.


## V. Supplementary Figures

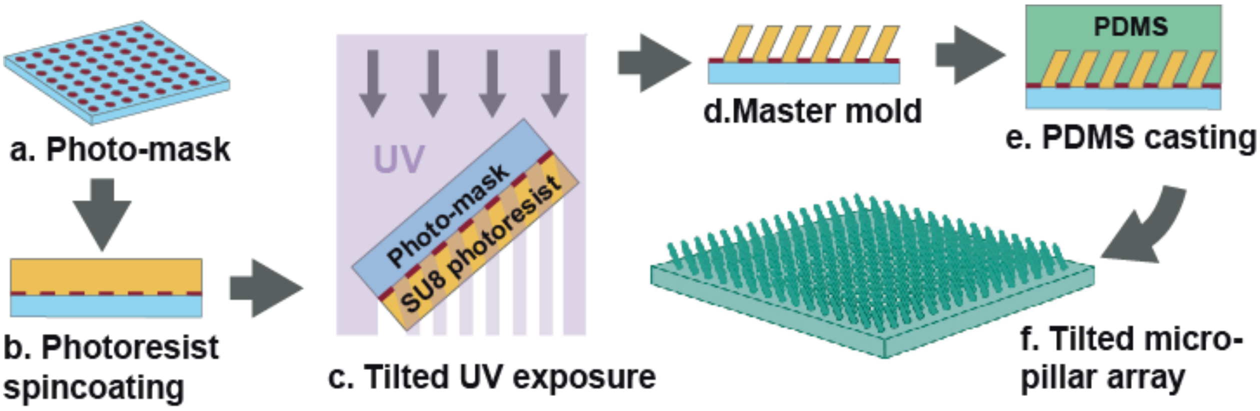


Supplementary Figure 1: Device fabrication process. See methods section for more details.

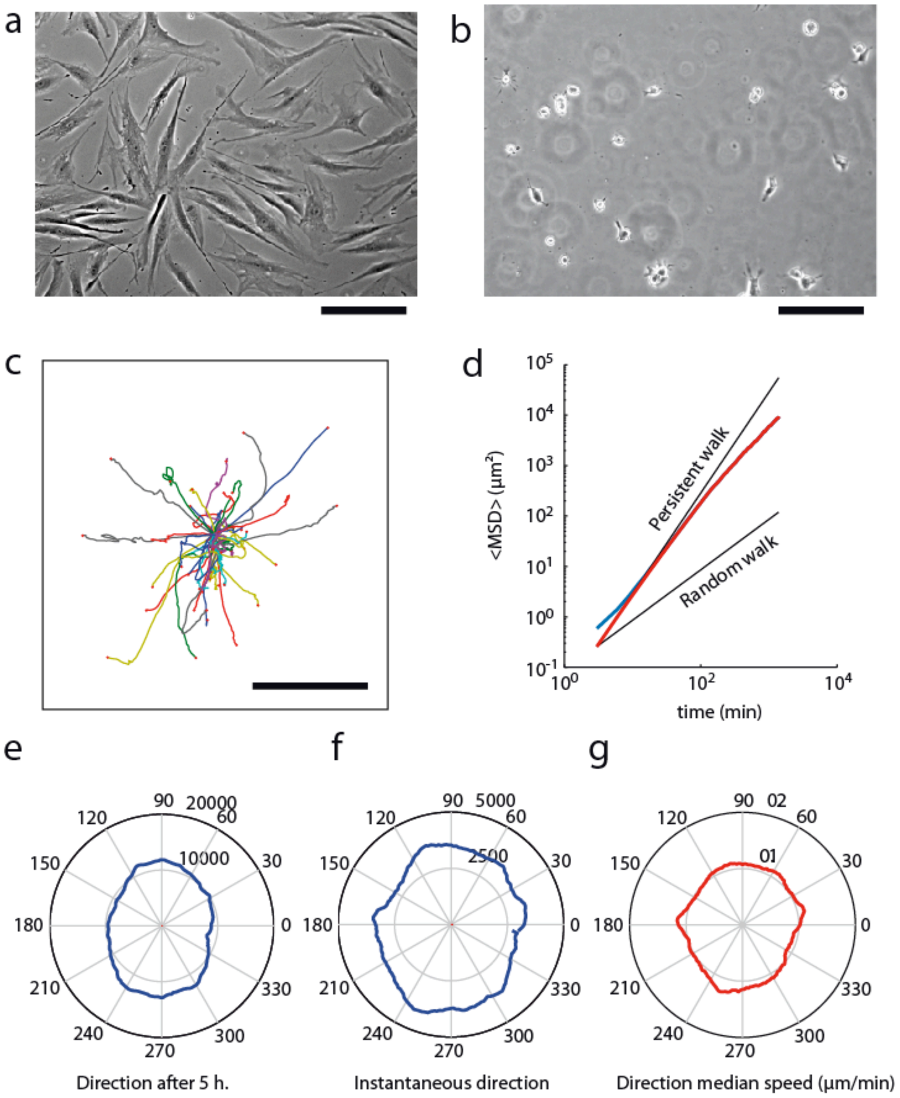


**Supplementary Fig. 2: Control experiments.** for cell adhesion and for isotropic Persistent Random Walk of NHDF cells confined under a non-adhesive flat substrate. **a,** Phase contrast image of NHDFs 24h after cells were seeded on a PDMS substrate treated with a 50 µg/mL Fibronectin solution. Cells adhered and spread on the substrate. Note that cell density is not representative of the one used in the migration assays analyzed in the paper. **b,** Phase contrast image of NHDFs 24 h after cells were seeded on a PDMS substrate treated with a 500µg/mL pLL-g-PEG solution. Cells did not adhere and remained round. **c,** Typical tracks of cells moving on an adhesive plastic substrate (treated with a 25 µg/ml fibronectin solution for 30 min) and confined with a non-adhesive flat PDMS substrate (treated with a 500 µg/ml pLL-g-PEG solution for 30 min after activation of the surface with plasma). All tracks start at the origin of the graph. **d,** Corresponding Mean Square Displacement (MSD). Red line shows the experimental mean MSD (filtered tracks, blue line corresponds to MSD of non-filtered tracks. See Methods section 5 for details) and black lines indicate limits of a fully persistent walk and a fully random walk. **e,** Angle histogram of the migration angle after 5 hours (n = 84572 single steps). **f,** Angle histogram of the instantaneous direction of migration. (n = 113037 single steps) **g,** median speed as a function of the instantaneous direction of migration on the

same data set. In (b-e), N = 293 cells from 18 movies. Scale bars are 200 μm in (a,b) and 100 μm in (c).

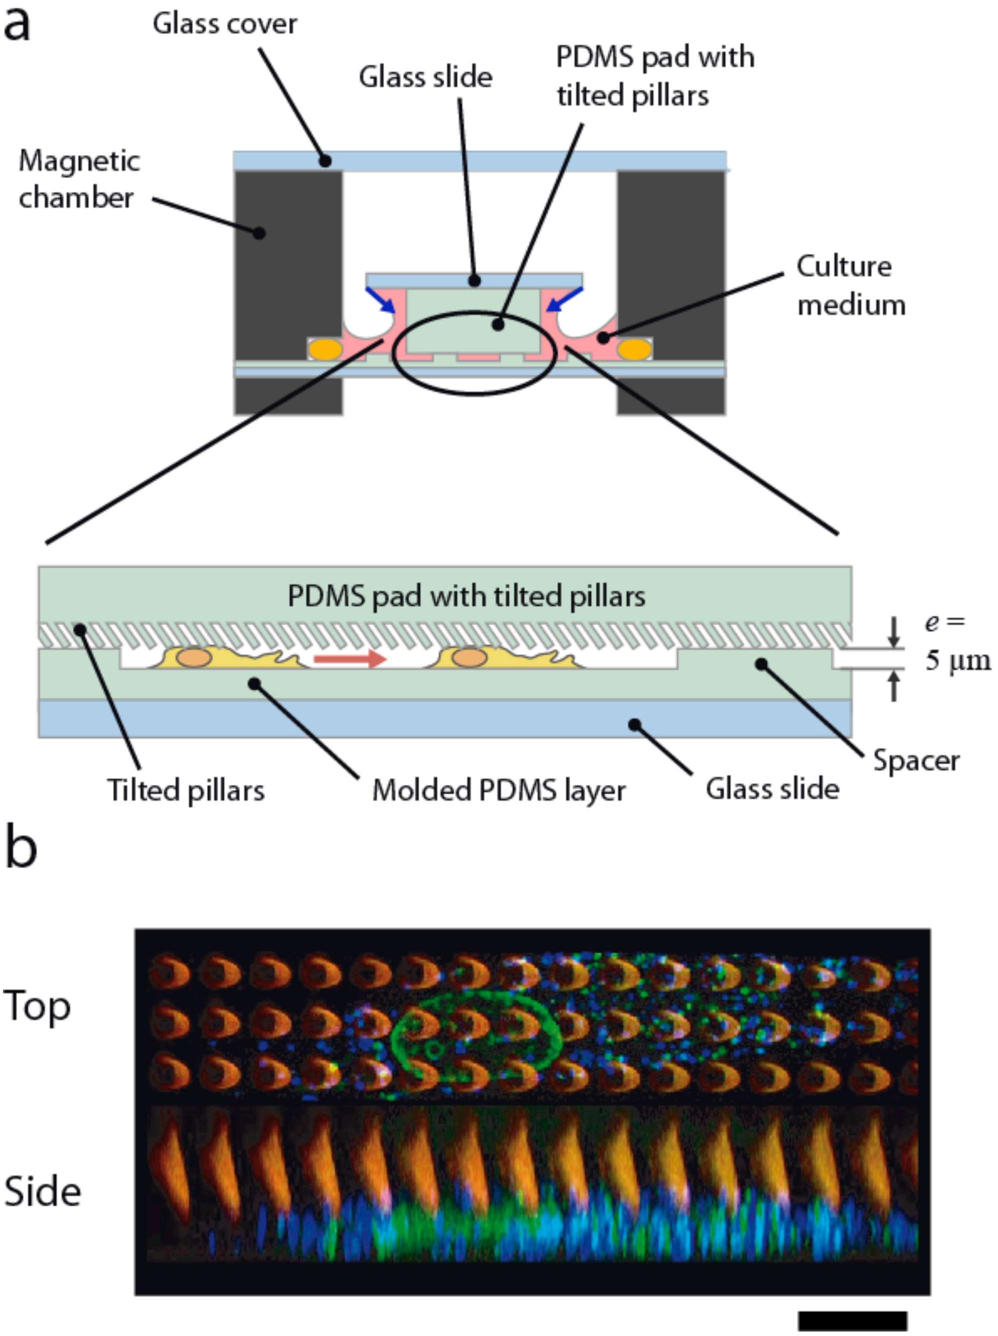


**Supplementary Figure 3: Cell migration under tilted pillars. a,** Schematic of the setup used to confine cells: cells were seeded on a thin microscope glass slide covered by a layer of PDMS in which large pillars (220 µm diameter, 5 µm thick) had been molded to ensure a precise spacing between pillars and the culture substrate. The top PDMS pad with the tilted pillars was maintained on the cells thanks to capillary forces after it was lain on the cells with a minimal amount of medium. **b.** Top and side views from a 3D reconstruction of a confocal fluorescence image stack. Orange shows fluorescent pLL-g-PEG staining of tilted pillars (pLL-g-PEG-Alexa594), green shows DRAQ5 staining (DNA) and blue shows WGA-FITC staining (cell membrane).

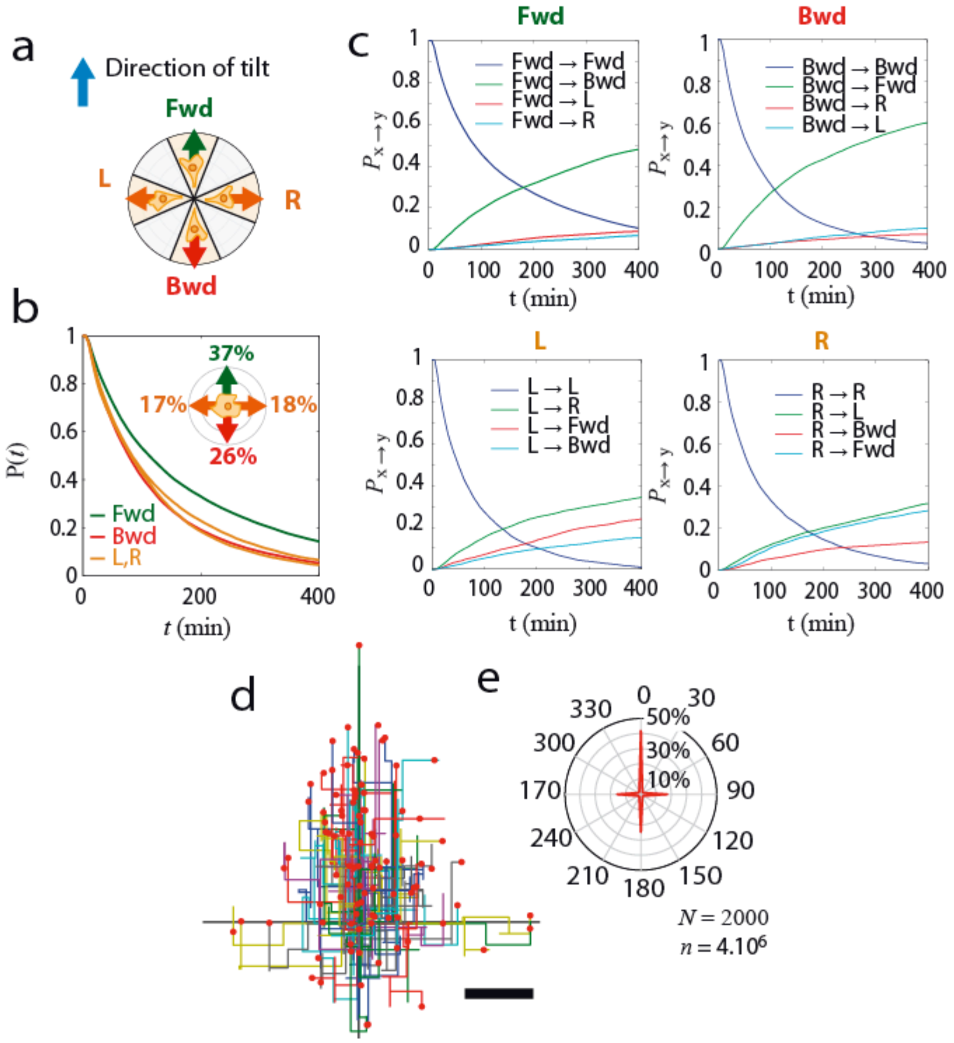


**Supplementary Figure 4: Quantification of turning behavior of cells under tilted pillars**. **a,** Definition of directions used in b-c. A cell is counted for an axis when its angle of migration is within ±π/8 around this axis. **b,** Probability of cells continuing in the same direction, for each initial direction (n = 22511, 12591, 6669, 9587 single steps for Fwd, Bwd, L, and R directions respectively). Insert shows the mean probabilities of turning towards a given direction. Probabilities were calculated from values in Supplementary table 1. **c**, Each graph represents, for cells initially moving in one of the four directions of the pillar lattice (Fwd, Bwd, L, R, see Figure 3c), the probability that cells remained in the same direction (dark blue curves, corresponding to curves shown in Fig. 3d) and the cumulative probability that cells turned in the other directions. For this calculation, a change of direction corresponds to a turn from an angle close to a given axis of the pillars lattice (±π/4) to an angle close to another axis. These distributions are based on all data points from high speed phases of cell tracks ($v$ > 50 nm/min) showing one of these specific directions of motion (n = 22511, 12591, 6669, 9587 for Fwd, Bwd, L, R, directions respectively). Changes of direction lasting less than 20 min were not taken into account to avoid "undecided" cells (cells which change their direction of migration many times consecutively) to dominate the distribution. **e,** Simulated trajectories from random walks corresponding to 16h, using measured parameters for speed, persistence and turning angle. **f,** Angle histogram of the instantaneous direction of migration of simulated cells. (N = 2000 cells, n = $4.10^6$).

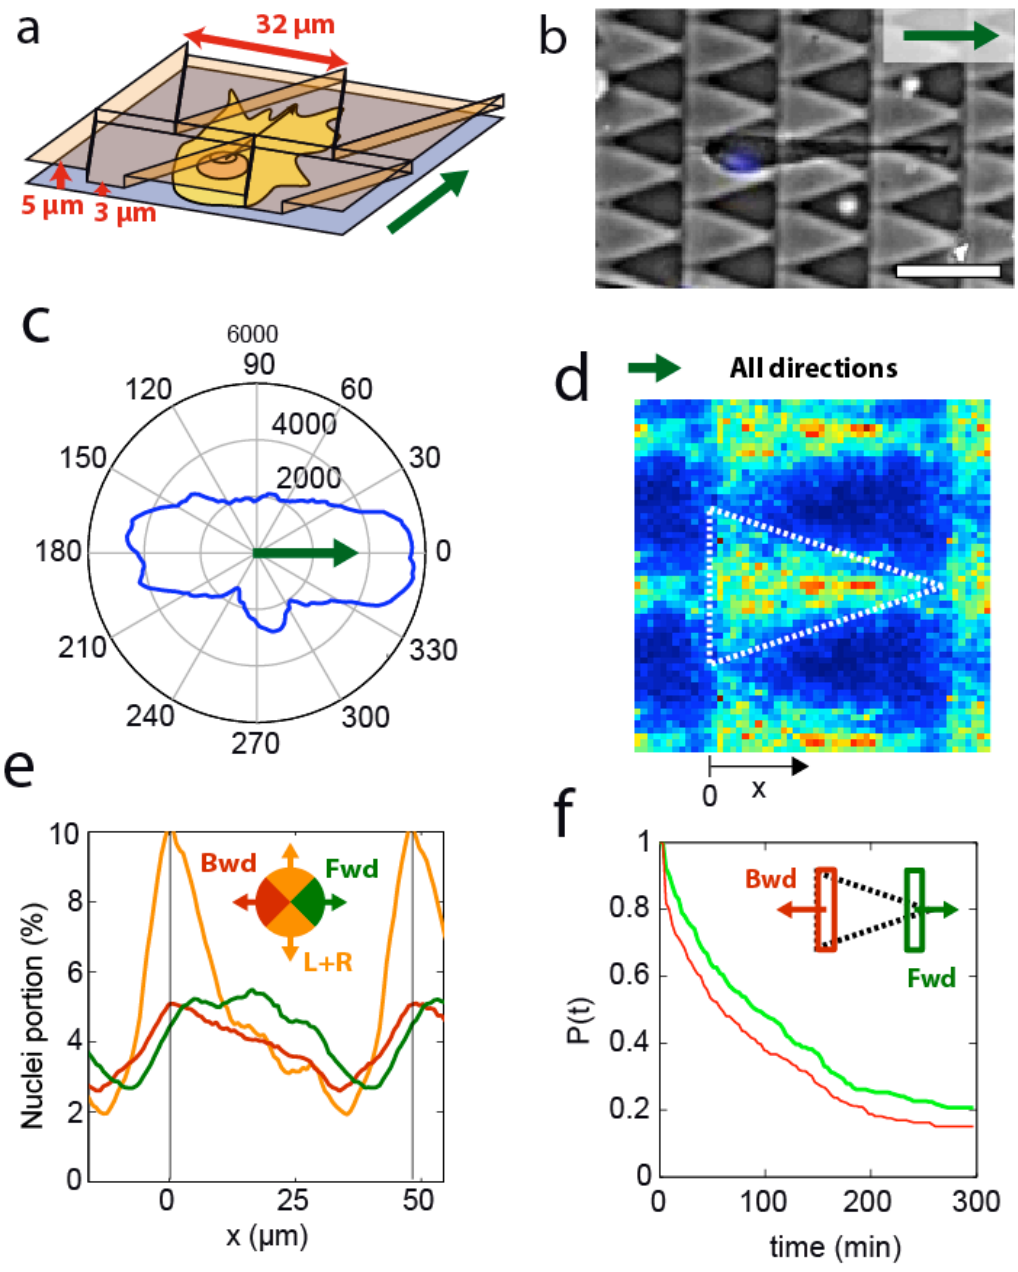


**Supplementary Figure 5: Biased migration under micro-prisms. a,** schematic diagram of the experiment. **b,** Overlay of phase contrast image and HOECHST staining (nucleus, blue) of a NHDF cell confined under micro-prisms. In this image, lighter triangles are deeper than darker triangles. Scale bar is 50 µm. **c,** histogram of the migration angle after 7.5 hours (n = 24413 single steps). **d,** Distribution maps of the center of mass of nuclei under the structures (n = 44622). The dashed triangle indicates the position of the hollow prism. **e,** distribution of nuclei along the *x* axis for the 4 main directions of migration (here, ordinate gives the portion of nuclei relatively to all nuclei measured in all direction) . Vertical lines indicate the position of the prism basis. **f,** Probability of the nucleus to remain in the same direction measured on nuclei located at the basis and at the tips of the prism. Inset shows the location of nuclei and the direction of motion took into account. In (a-f), the green arrow indicates the direction of the prism tip. Data are from 145 cell tracks from 16 movies.

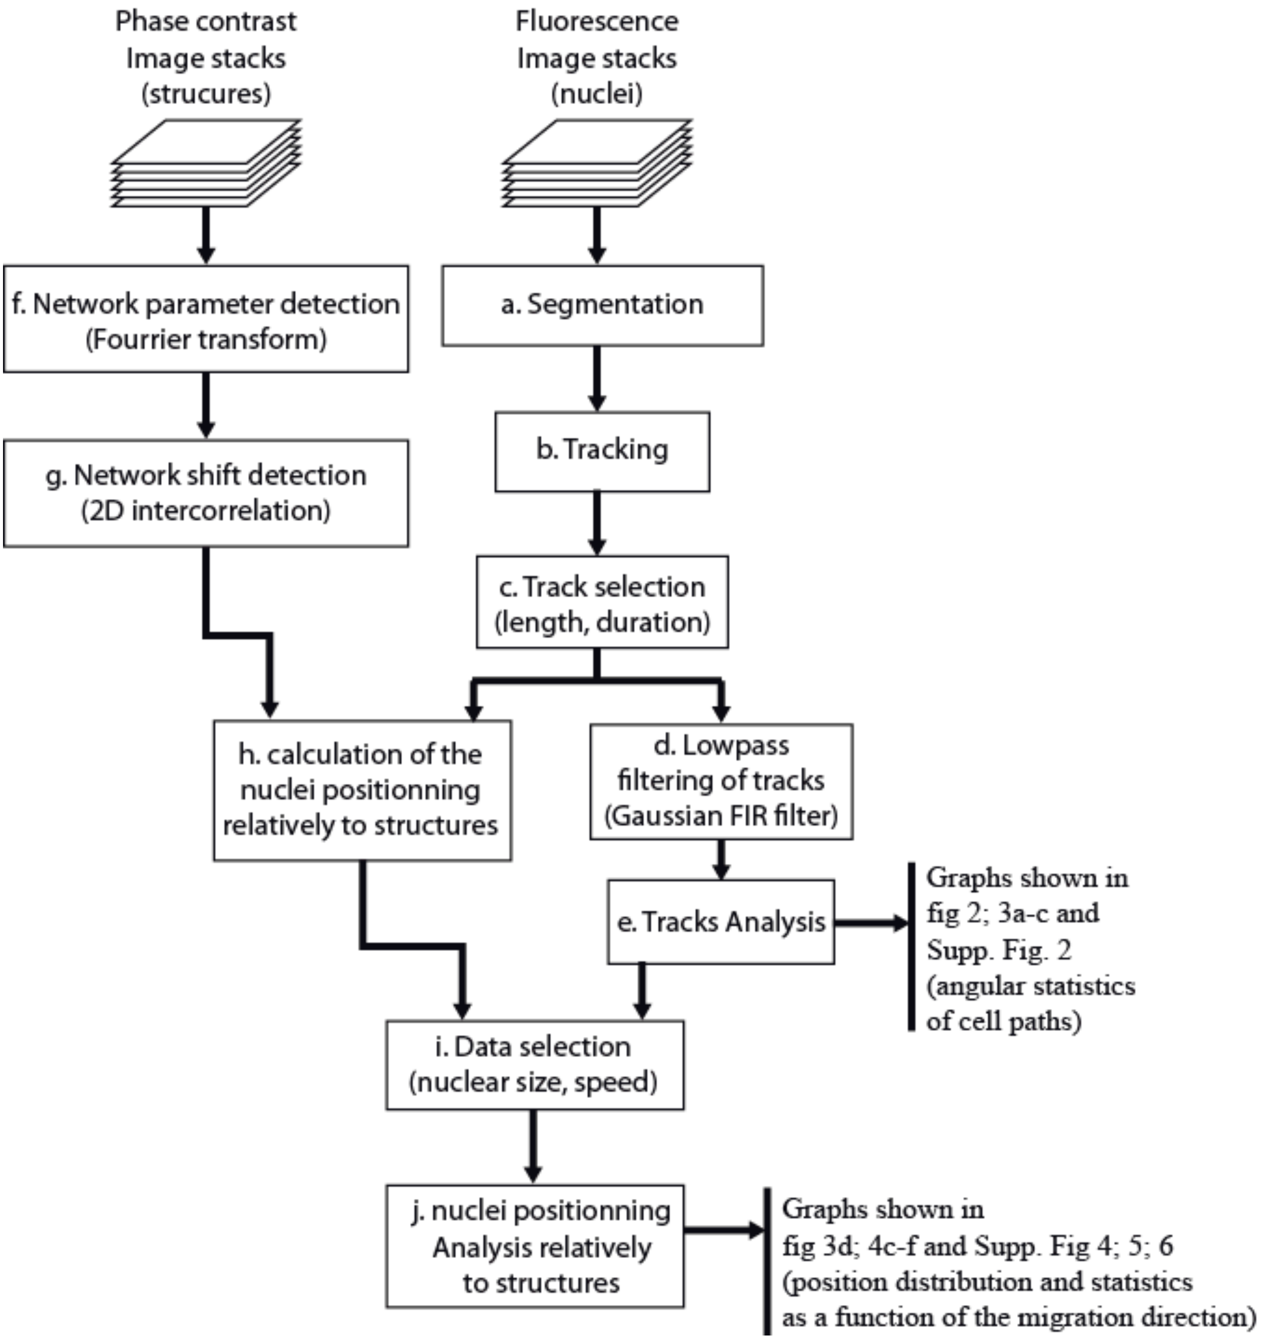


**Supplementary Figure 6:** Schematic diagram of the automated analysis program (see methods section for details.

**VI. Author contributions**

J. Hu and Y. Chen did the micro-fabrication and characterisation of the micropillars by SEM, Y.-J. Liu designed and performed all cell experiments, fabricated the micro-prisms and performed some data analysis, O. Benichou and R. Voituriez developed the theoretical model and M. Le Berre did the data analysis, statistics and simulations, with the help of P. Maiuri. M. Le Berre, R. Voituriez and M. Piel were the main writers of the manuscript.
